# Supplementary material for: ArchGym: An Open-Source Gymnasium for Machine Learning Assisted Architecture Design
Source: arXiv:2306.08888 source file (2023-06-15)
Supplement: Supplementary file 1 [file appendix.tex]

%\section*{Appendix}

%In Figure~\ref{fig:arch_dse_problem}, we provide the parameter-set for each \ours environment and elaborate on our experimental setup, which we deferred from the main section of the paper to avoid distracting the reader from the main focus of the contribution. Briefly, we use three environments to demonstrate the utility of \ours and their details (architecture, parameters, workloads) are illustrated. 
% Furthermore, simulator, workload, and interface signals (action, observation, reward) are tabulated in Table~\ref{tab:gymenv_summary} for each environment.



% \subsubsection{\textbf{Memory Controller}}

% In our \textsc{DRAMGym} environment, the objective is to optimize the memory sub-system using AI/ML agents. To that end, memory controller is a key component that affects the performance of the system. Our goal is to design a memory controller for three different objectives -- (a) Low latency, (b) Low Power, (c) Low latency and low power. These are realistic objectives depending on the target domain. For instance, in an embedded use case, achieving low power might be critical, whereas achieving low latency in a high-performance computing domain is critical. 

% \niparagraph{Simulator and parameters.}
% To simulate our DRAM Memory controller we use DRAMSys~\cite{dramsys}. This simulator provides many parameters to configure the memory controller such as \texttt{RefreshPolicy}, \texttt{RequestBufferSize}, and \texttt{MaxActiveTransactions} to name a few. For the full list of parameters for the memory controller see Figure~\ref{fig:arch_dse_problem}.

% \niparagraph{Workload.} From a DRAM perspective, a workload is a set of memory read/write accesses. Thus, we pick two extreme access patterns in this context: a streaming memory access trace and a random memory access trace. These are representative of real-world workloads. For instance, dense matrix-matrix multiplication and convolution operations would result in streaming access. Likewise, operations like pointer chasing and sparse matrix-matrix multiplication will result in random memory access.

% % \textbf{Optimization Objective.} 
% % Our goal is to design a memory controller for three different objectives -- (a) Low latency, (b) Low Power, (c) Low latency and low power. %In this work, we target two memory traces: streaming address and random address memory trace. 
% % These are realistic objectives depending on the target domain. For instance, in an embedded use case, achieving low power might be critical, whereas achieving low latency in a high-performance computing domain is critical. We want to compare the performance of single-agent RL with multi-agent RL formulations against these optimization objectives.

% % \textit{Observations.} In this version of the DRAM-Gym environment, the observation is a tuple of \texttt{<latency, power, energy>}. This observation is similar to a multigrid world environment where the objective is to reach a specific coordinate. In our case, the coordinates are an n-dimensional parameter space where each combination of the parameter space will have a corresponding \texttt{<latency, power, energy>}. We aim to find the specific coordinates in the n-dimensional space (i.e., memory controller parameters) that satisfy the optimization objectives.

% % \textit{Actions.} The considered action space corresponds to the parameters in the memory controller. The action space is diverse; some actions are categorical variables (e.g., \texttt{Page policy}), and some are integers (e.g., \texttt{Request Buffer Size}). For more information on the parameter space for the memory controller we explore in this work, we refer the readers to Table~\ref{tab:mc_params}.

% % \textit{Rewards.}  We use similar reward structure for the objective of minimizing power and latency. For minimizing both, we use the following reward function
% % \begin{equation}
% % \centering
% % r_{x} = \frac{X_{\text{target}}}{|X_{\text{target}}-X_{\text{obs}}|} \, , \label{eq:r_power}
% % \end{equation}
% % \label{reward_formula}
% % where $X_{\text{target}}$ is the target power/latency and $X_{\text{obs}}$ is the currently-achieved value.
% % For the joint objective of minimizing both power and latency, we take the product of $r_{\text{joint}} = r_{\text{power}}*r_{\text{latency}}$.

% % \niparagraph{Workloads.} From a DRAM perspective, a workload is a set of read/write accesses for a given application. Thus, we pick two extreme access patterns in this context, namely a streaming memory access trace and random memory access trace. Both choices are representative for many applications. For instance, convolution operations (machine learning), matrix-matrix multiplication in HPC, often have streaming like access pattern.

% % Likewise, the random memory access trace are also representative to many applications. For instance, system-level optimizations exploit sparsity~\cite{sparse-nn,sparse-2}. To avoid multiplying zeros (to save latency, energy), only the indices of the non-zero elements are stored and accessed. Since it is hard to determine the exact indices of non-zero elements in a matrix during runtime, multiplying two sparse matrices will result in a non-deterministic random access pattern as shown in \Fig{fig:random} Another example, is many applications have scatter-gather operations which results in random access patterns.



% \subsubsection{\textbf{DNN Accelerator}}
% In our \textsc{TimeloopGym} environment, the objective is to optimize the compute in addition to the memory component for dedicated DNN hardware using the agents. 
% The coupled structuring of processing elements (PEs) and memory hierarchy in accelerators impacts how efficiently the specialized hardware performs its task. 

% Similar to \textsc{DRAMGym}, our goal is to design a DNN accelerator for the following individual objectives: (a) Energy efficiency, (b) Low latency, (c) Small die area, and (d) a combination of all three.

% % \paragraph{Actions}
% % The action space in which the agent makes decisions corresponds to the architectural parameters listed in Table ~\ref{fig:arch_dse_problem}. The accelerator architecture attempts to closely model Eyeriss~\cite{chen2016eyeriss} using Timeloop~\cite{parashar2019timeloop}. These parameters tune features of the accelerator memory hierarchy (e.g. depth, blocks, etc.) as well as the dimensions of the spatial PE array for compute, both of which have implications on the system's overall performance for a specific workload. 
% \niparagraph{Simulator and parameters.}
% Our DNN accelerator design closely modeled Eyeriss~\cite{chen2016eyeriss} and is simulated using Timeloop~\cite{parashar2019timeloop}. Some of the available parameters for tuning include \texttt{NumPEs}, \texttt{WeightsSPad\_MemoryDepth}, and \texttt{SharedGlobalBuffer\_NumBanks}. For the full list of parameters explored for the Eyeriss-like accelerator see Figure~\ref{fig:arch_dse_problem}.

% \niparagraph{Workloads}
% In the case of DNN acclerators, a workload is simply a neural network model. More specifically, in the context of an accelerator like Eyeriss, our workloads need to be convolutional neural networks (CNNs). We selected three CNNs for our evaluation: AlexNet, MobileNet, and ResNet-50. These models present differing degrees of model size and complexity suitable for various domains. 

% % \paragraph{Observations}
% % In our implementation of the TimeloopGym environment, the observation is a tuple of \texttt{<latency, energy, area>}. Each point in the architectural design space (see parameters in Table ~\ref{fig:arch_dse_problem}) has a corresponding tuple. Our work focuses on the architectural design problem and disregards designs that do not have valid mappings, returning a poor observation in these cases. 
% % \paragraph{Rewards}
% % The same reward formulation is used for minimizing energy, latency and, area as the equation in Section ~\ref{reward_formula} where $X_{\text{target}}$ in TimeloopGym's context is the target energy, area, or latency and $X_{\text{obs}}$ is the measured value.
% % For minimizing the joint objective of energy, latency, and area, we once again take the product of $r_{\text{joint}} = r_{\text{energy}}*r_{\text{latency}}*r_{\text{area}}$.


% \subsubsection{\textbf{System On-Chip}}
% Finally in \textsc{FARSIGym}, the goal is to optimize the entire \emph{system}, including compute, memory, and interconnects. System On-Chips (SoC) include many heterogeneous hardware blocks (e.g, CPU, DSP, accelerator, etc.) and memory (e.g., Flash, ROM, RAM, etc.) that must talk to each other via interconnects and the exact allocation of these components introduces different design points with performance trade-offs.  

% % \paragraph{Actions} The action space in which the agent makes
% % decisions corresponds to the architectural parameters listed in
% % Table~\ref{fig:arch_dse_problem}. These parameters tune features of the PE (e.g. Type,
% % Frequency, count, etc.), NoC and Memory, all of which have implications on the SoC’s
% % overall design performance for a specific workload.

% % \paragraph{Rewards}
% % We use reward structure for the objective
% % of minimizing power, latency and area. For minimizing both, we use the following reward function.

% % reward function is quantified
% % using their design's (metric) normalized distance to budget
% % with a dampening factor to the metrics already meeting budget (Equation~\ref{eq:dist}). $m$, $D_m$, $B_m$ and $\alpha$ denote, a metric, design value for the metric, budget value for that metric, and dampening factor when the budget is met. 
% % \begin{align} \label{eq:dist}
% %     & distance\ to\ budget = \sum_m \alpha*\frac{(D_m - B_m)}{B_m}\\
% %     & m \in \{ Performance, Power, Area\} \nonumber
% % \end{align}

% % If no improved designs are found, we inform the system generation stage for the next iteration to target the task/block with the next highest distance (comparing to the last).

% % minimizing power
% % \paragraph{Observations}
% \niparagraph{Simulator and parameters.}
% To simulate an SoC we use FARSI~\cite{boroujerdian2022farsi}. This system-level simulator provides configurable SoC parameters such as \texttt{PE\_Count}, \texttt{NoC\_Freq}, and \texttt{Mem\_BusWidth}. For the full list of parameters for the SoC see Figure~\ref{fig:arch_dse_problem}. It should be noted that we solve the resource allocation problem as well as workload mapping
% problem in this environment.

% \niparagraph{Workloads}
% For the FARSI workload analysis, we use the AR domain workloads (Task Dependency Graph or TDG) in its provided database.
% % with the characteristics of the domain’s workloads (Task Dependency Graph or TDG) and the PPA (power, performance and Area) estimates of the individual PEs. 
% In the TDGs, tasks constitute the smallest unit of optimization and are selected as they significantly impact the system behavior.  
% % Power and area estimations of PE is done using AccelSeeker \cite{}, and for NoCs and memory, CACTI \cite{} is used. 
% The rigid constraints of the AR domain demand accelerator-rich and complex domain-specific SoCs. We target the primitive workloads, i.e., audio and image processing, as they are present in almost any AR/VR application.
% %
% % Audio Decoder (Audio) is used to playback the audio based on the user pose. It has 15 tasks and uses both loop and task level parallelism (highest TaLP among all) and is from a newly released AR/VR testbed [16]. CAVA [49] processes raw images from sensors to feed the vision backend (e.g., a CNN). It has seven stages with loop level parallelism. Edge Detection (ED) [24] has six stages and has both task and (high) LLP. It is the most communication-intensive benchmark.
